# Supplementary material for: Phase Stability and Raman/IR Signatures of Ni-Doped MoS$_2$ from Density-Functional Theory Studies
Source: arXiv:2010.02198 ancillary file (2021-02-28)
Supplement: Supplementary file 1 [file SI.pdf]

# Supporting Information: Phase stability and Raman/IR signatures of Ni-doped $MoS_2$ from DFT studies

Enrique Guerrero, Rijan Karkee, and David A. Strubbe*

*Department of Physics, University of California, Merced, Merced, CA 95343*

E-mail: dstrubbe@ucmerced.edu

# Convex hull phase diagram calculations

Convex hull plots were calculated using the function `ConvexHullMesh` in `Mathematica v12.1`.[S1] In some cases, the computed convex hull was incorrectly computed by Mathematica to not encompass points that are very close to the convex hull faces. We found that including extra arbitrary points far above the hull in energy resolved this issue.

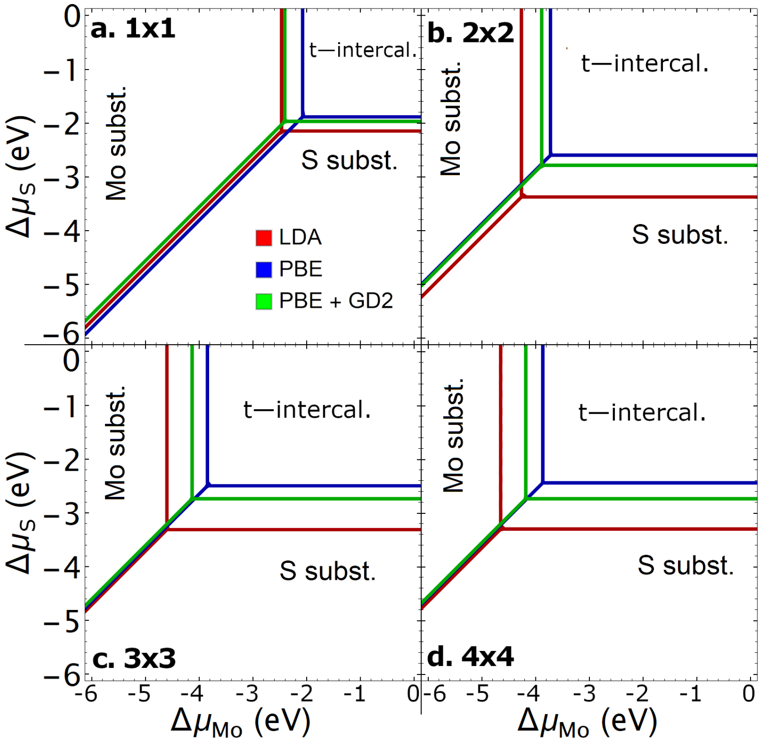


Figure S1: Phase diagrams for LDA, PBE, and PBE+GD2. The difference between functionals is similar across sizes, with LDA triple points residing at further negative $\Delta\mu_{\mathrm{S}}$ and $\Delta\mu_{\mathrm{Mo}}$ than PBE. There is little difference between the 3×3 and 4×4 diagrams, indicating the plot is converged with respect to Ni concentration.

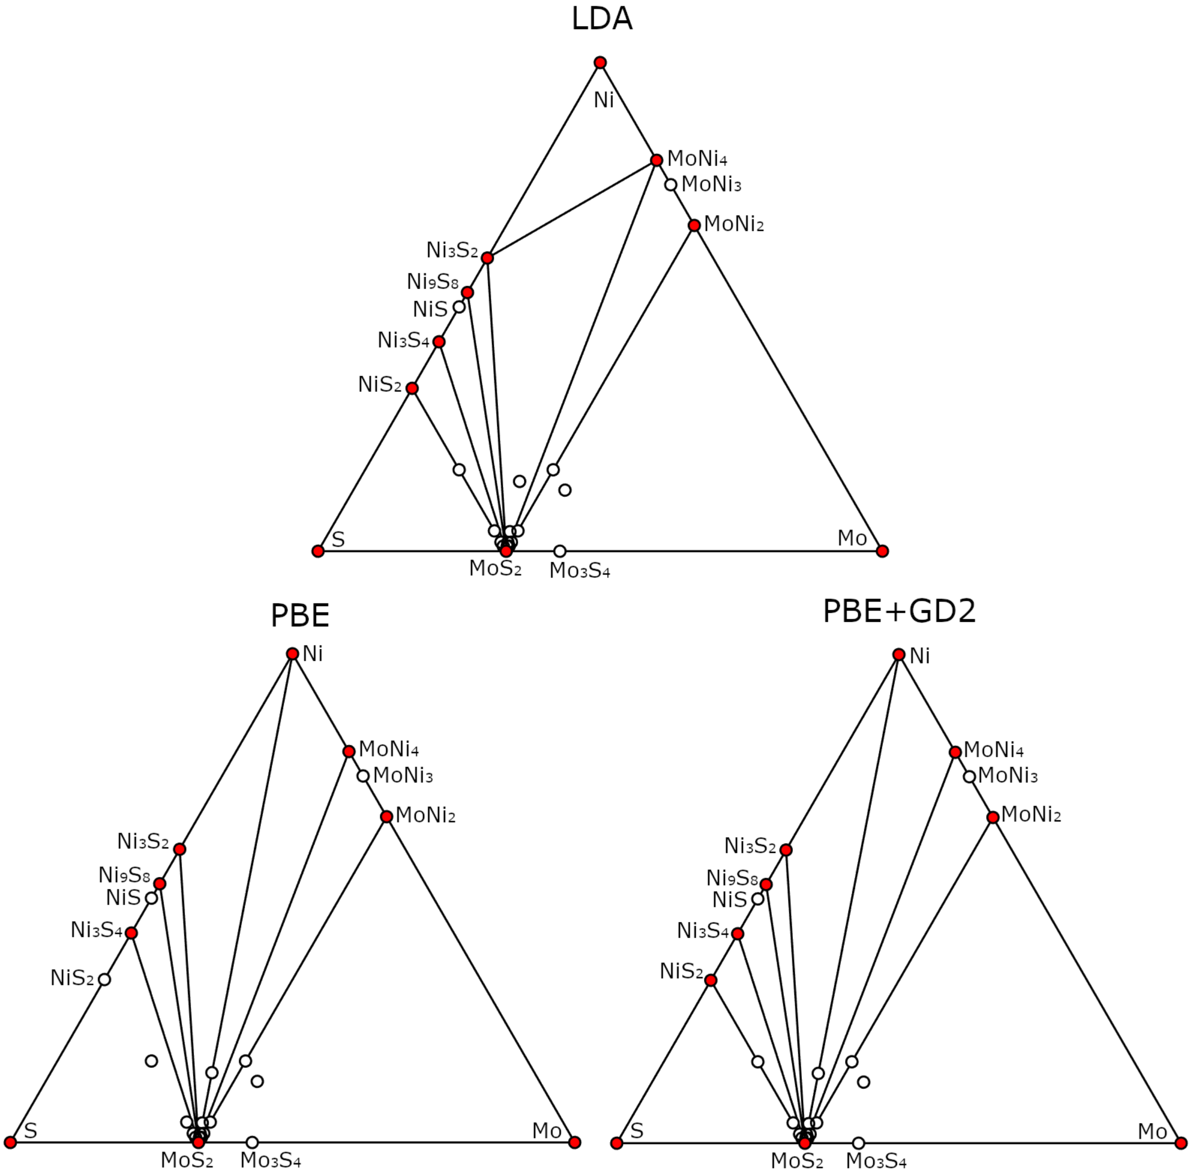


Figure S2: Convex hull diagrams for LDA, PBE, and PBE+GD2. Although the relative energy differences between these three comparisons are small, qualitative changes to the convex hull are substantial. Red filled-in circles represent structures which are on the convex hull line and are thus the most stable structures at $T = 0$ K. The line between $MoS_2$ and $NiS_2$ (which contains the Mo-substituted structures) is on the convex hull when using LDA and PBE+GD2, but not for PBE alone. The line between $MoS_2$ and Ni is not on the convex hull in LDA. Intercalated structures are above the convex hull edge in energy.

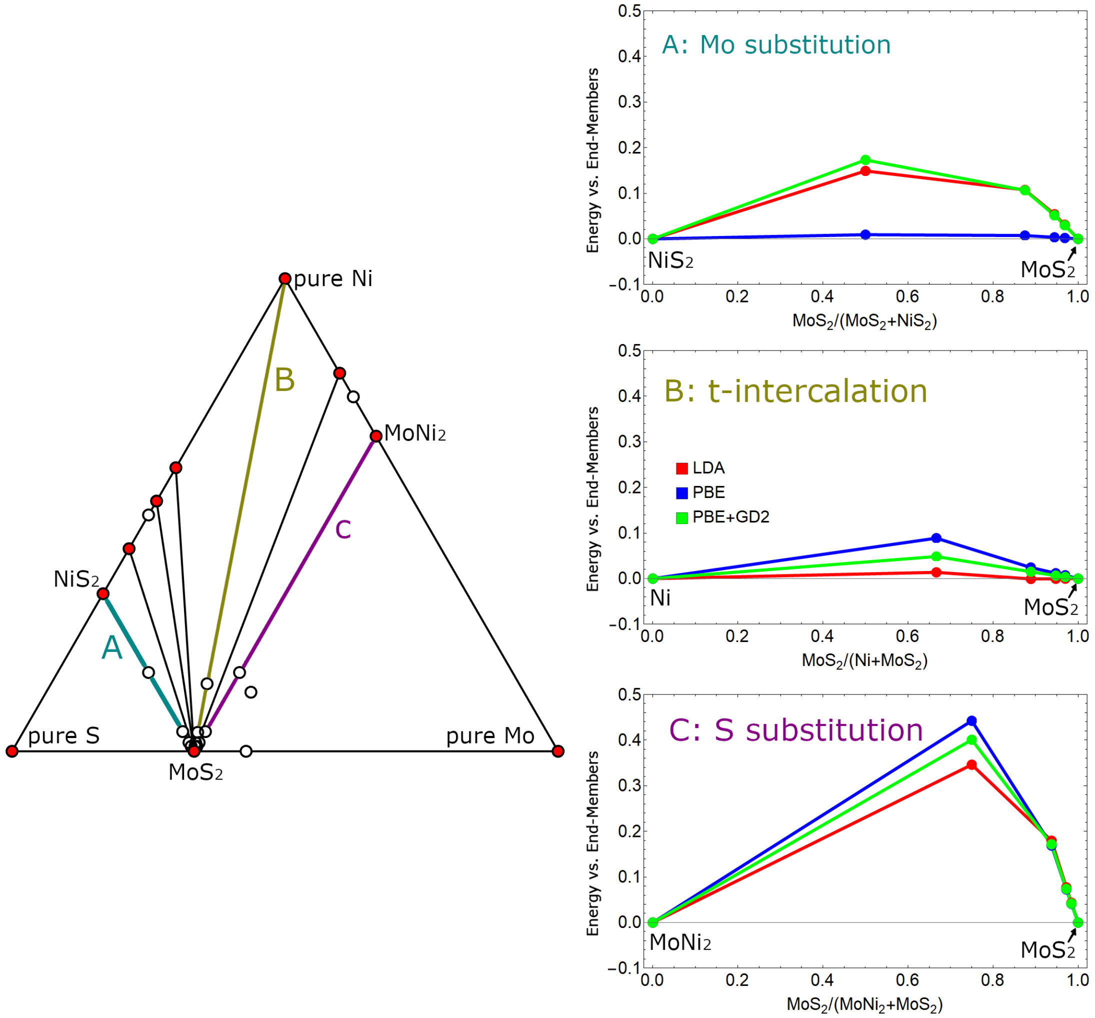


Figure S3: 1D convex hull diagrams from $MoS_2$ to: $NiS_2$ (Mo substitution, A), pure Ni (intercalation, B), and $MoNi_2$ (S substitution, C). The $x$-axis (energy $= 0$) is always below the calculated structures, so it always constitutes the convex hull. These 1D convex hull diagrams (with energy in eV per atom) are comparable to previous literature on V, Te, and Mo ternary 2D alloys.[S3] PBE behaves differently along the Mo substitution line, but overall the results are similar for the different functionals. T-intercalated energies are close to the convex hull line.

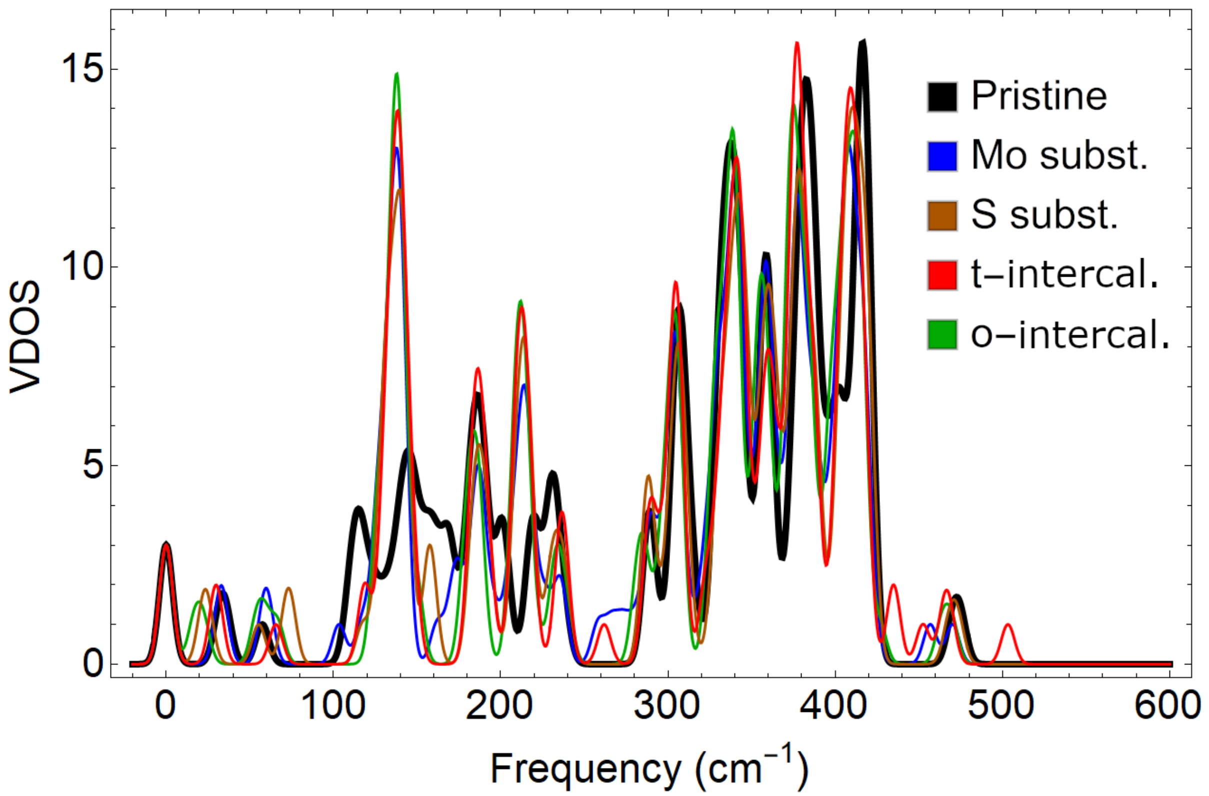


Figure S4: Vibrational density of states (VDOS) for doped structures using Gaussian broadening of 4 cm$^{-1}$. Doped structures are 3×3 supercells computed at $q = \Gamma$. The pristine case is a primitive cell calculated on a corresponding 3×3×1 $q$-grid. This data can be used to identify the origin of Raman/IR peaks in doped $MoS_2$.

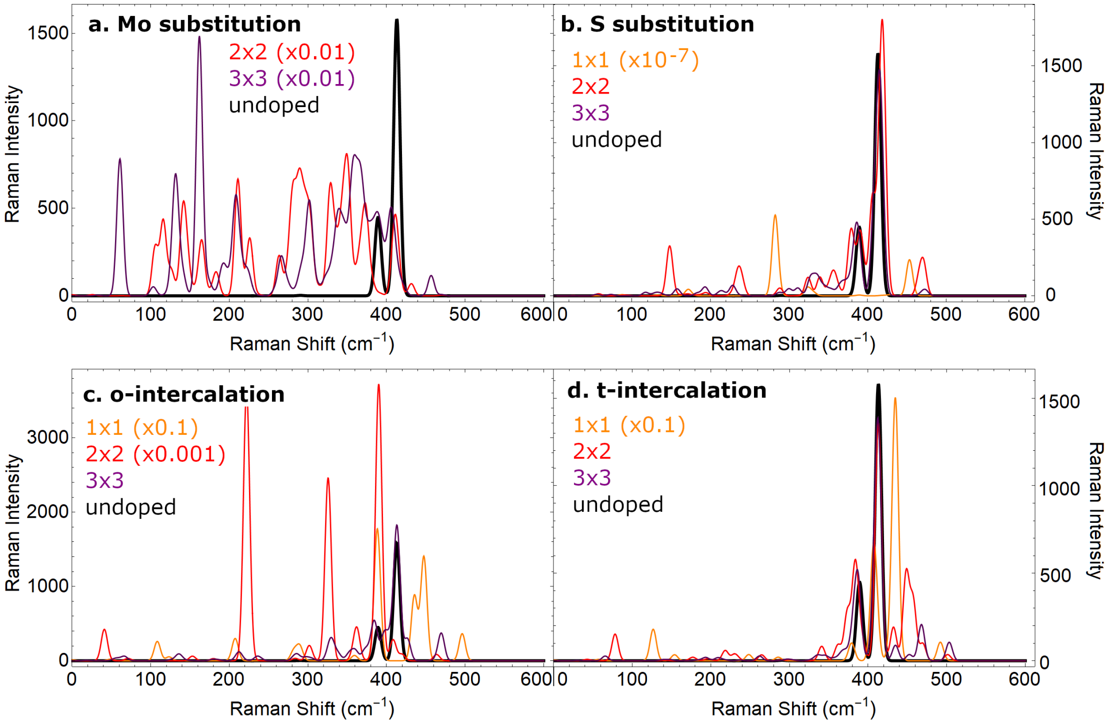


Figure S5: Raman spectra, in $A^4$/amu per $MoS_2$ unit, for types of doping as a function of supercell size. Gaussian broadening of 4 $cm^{-1}$ was used. Some spectra were too intense to fit in the plot, so they were scaled by the factor in the legend. $1 \times 1$ Mo substitution was metallic and so the dielectric calculation could not be done by DFPT.

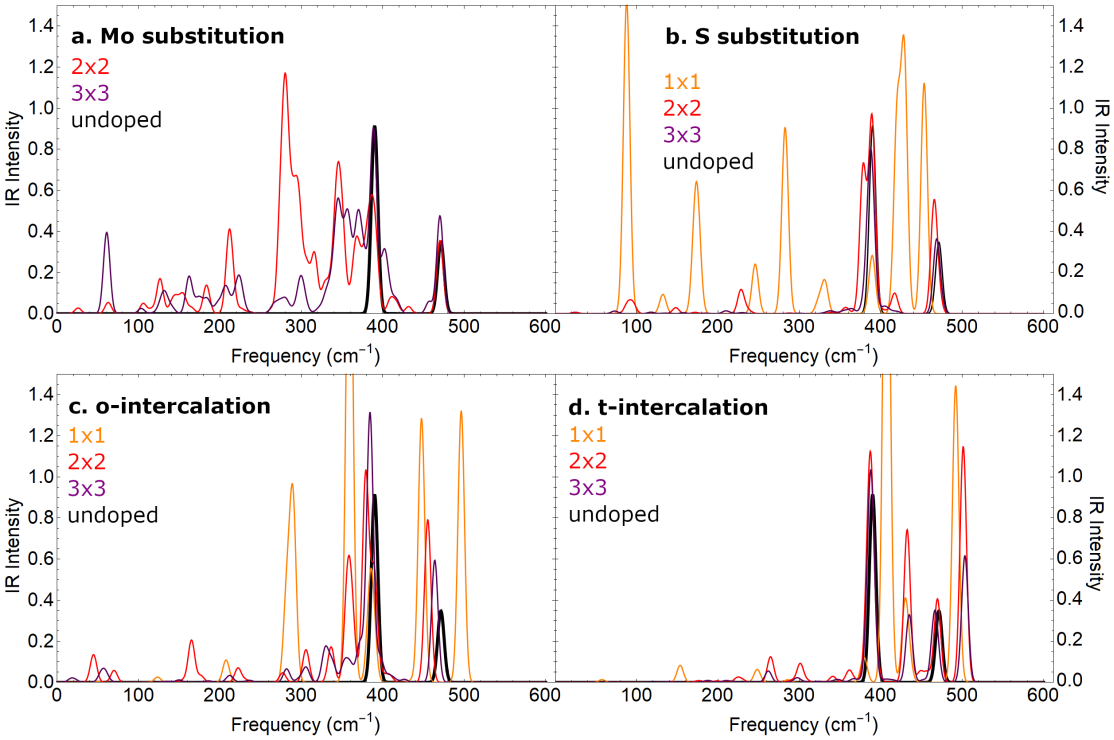


Figure S6: IR spectra in $(D/A)^2$/amu per $MoS_2$ unit for types of doping as a function of supercell size. Gaussian broadening of 4 $cm^{-1}$ was used.

**Table S1: Structure Information for Reference Crystals Containing Mo, Ni, and S**

| Formula | Materials Project ID | Spacegroup | Smearing used? | $k$-grid | $a$, $b$, $c$ (Å) | $\alpha, \beta, \gamma$ (°) |
|---|---|---|---|---|---|---|
| Mo | mp-129 | Im$\overline{3}$m | yes | $6 \times 6 \times 6$ | 3.1521, 3.1521, 3.1521 | 90.000, 90.000, 90.000 |
| Ni | mp-23 | Fm$\overline{3}$m | yes | $6 \times 6 \times 6$ | 2.4490, 2.4489, 2.4489 | 59.4061, 59.4040, 59.4040 |
| S | mp-557869 | P$2_1$ | no | $3 \times 3 \times 3$ | 10.942, 10.8158, 11.2184 | 90.0000, 96.4411, 90.0000 |
| $MoS_2$ | mp-2815 | P$6_3$/mmc | no | $6 \times 6 \times 4$ | 3.1902, 3.1902, 12.4159 | 90.0000, 90.0000, 119.9715 |
| $Mo_3S_4$ | mp-2164 | R$\overline{3}$ | no | $6 \times 6 \times 6$ | 6.4291, 6.4291, 6.4291 | 91.2731, 91.2740, 91.2740 |
| $Ni_2Mo$ | mp-784630 | Immm | yes | $6 \times 6 \times 6$ | 4.4095, 4.4095, 4.4095 | 146.4497, 130.9693, 60.7215 |
| $Ni_3Mo$ | mp-11506 | Pmmn | yes | $6 \times 6 \times 6$ | 4.1479, 4.3523, 5.0519 | 90.0005, 89.9999, 89.9999 |
| $Ni_4Mo$ | mp-11507 | I4/m | no | $6 \times 6 \times 6$ | 3.4925, 4.3640, 4.3644 | 80.7960, 66.3502, 66.4451 |
| $NiS_2$ | mp-2282 | Pa$\overline{3}$ | yes | $6 \times 6 \times 6$ | 5.5825, 5.5825, 5.5825 | 90.0000, 90.0000, 90.0001 |
| $Ni_3S_4$ | mp-1050 | Fd$\overline{3}$m | no | $6 \times 6 \times 6$ | 6.6350, 6.6350, 6.6350 | 119.9791, 89.9648, 60.0215 |
| NiS | mp-594 | P$6_3$/mmc | no | $4 \times 4 \times 4$ | 9.4448, 9.4448, 3.1478 | 89.9825, 90.0177, 119.9988 |
| $Ni_9S_8$ | mp-976920 | C222 | no | $2 \times 2 \times 2$ | 7.1951, 7.1951, 9.2704 | 89.9995, 90.0001, 79.7682 |
| $Ni_3S_2$ | mp-362 | R32 | no | $6 \times 6 \times 6$ | 4.0220, 4.0220, 4.0220 | 89.5796, 89.5795, 89.5793 |
| $NiMo_3S_4$ | mp-685980 | P$\overline{1}$ | no | $6 \times 6 \times 6$ | 6.3215, 6.4594, 6.4704 | 97.1060, 96.9479, 92.2066 |

PBE+GD2 computed structures. PBE structures can be found on the materials project website `materialsproject.org`.[S2] Gaussian smearing of $10^{-4}$ Ry was used where indicated. $k$-grid densities were fine enough to converge the final energies to within 0.01 eV per atom.

**Table S2: Structural Parameters of Ni-Doped $MoS_2$**

| | | undoped | Mo subst. | S subst. | t-intercal. | o-intercal. |
|---|---|---|---|---|---|---|
| a (Å) | 1 × 1 | 3.19 | 3.30 | 3.19 | 3.22 | 3.18 |
| | 2 × 2 | " | 3.20 | 3.18 | 3.20 | 3.19 |
| | 3 × 3 | " | 3.19 | 3.18 | 3.19 | 3.19 |
| | 4 × 4 | " | 3.20 | 3.19 | 3.19 | 3.19 |
| c (Å) | 1 × 1 | 12.4 | 11.3 | 10.8 | 12.6 | 12.5 |
| | 2 × 2 | " | 12.3 | 12.3 | 12.5 | 12.4 |
| | 3 × 3 | " | 12.4 | 12.3 | 12.5 | 12.4 |
| | 4 × 4 | " | 12.4 | 12.4 | 12.5 | 12.4 |
| Ni-S distances (Å) below 3.1 Å | | | | | | |
| | 1 × 1 | | 2.23 × 6 | 2.16 × 3 | 2.15 × 1, 2.18 × 3 | 2.38 × 2, 2.39 × 4 |
| | 2 × 2 | | 2.37 × 4, 2.38 × 2 | | 2.12 × 1, 2.17 × 3 | 2.36 × 4, 2.37 × 2 |
| | 3 × 3 | | 2.23 × 2, 2.25 × 2, 2.39 × 1 | | 2.12 × 1, 2.17 × 3 | 2.28 × 2, 2.29 × 1, 2.45 × 1, 2.48 × 2 |
| | 4 × 4 | | 2.22 × 2, 2.24 × 2, 2.42 × 1 | | 2.11 × 1, 2.17 × 3 | 2.26 × 1, 2.27 × 2, 2.50 × 3 |
| Ni-Mo distances (Å) below 3.1 Å | | | | | | |
| | 1 × 1 | | | 2.68 × 3, 2.78 × 1 | 2.76 × 1 | |
| | 2 × 2 | | | 2.55 × 3 | 2.61 × 1 | |
| | 3 × 3 | | 2.80 × 1, 2.82 × 1 | 2.56 × 3 | 2.59 × 1 | |
| | 4 × 4 | | 2.80 × 2 | 2.56 × 3 | 2.59 × 1 | |

Structural characteristics of relaxed PBE + GD2 Ni-doped $MoS_2$ structures are shown above. $a$ parameters are the average over the primitive cells in the supercell. Ni-S and Ni-Mo distances below 3.1 Å are shown multiplied by how many equal distances there are in a given structure.

**Table S3: Energies Above Hull (eV/atom)**

| Formula | LDA | PBE | PBE + GD2 |
|---|---|---|---|
| Mo | 0 | 0 | 0 |
| Ni | 0 | 0 | 0 |
| S | 0 | 0 | 0 |
| $MoS_2$ | 0 | 0 | 0 |
| $Mo_3S_4$ | 0.065 | 0.074 | 0.124 |
| $Ni_2Mo$ | 0 | 0 | 0 |
| $Ni_3Mo$ | 0.024 | 0.016 | 0.013 |
| $Ni_4Mo$ | 0 | 0 | 0 |
| $NiS_2$ | 0 | 0.021 | 0 |
| $Ni_3S_4$ | 0 | 0 | 0 |
| NiS | 0.018 | 0.022 | 0.014 |
| $Ni_9S_8$ | 0 | 0 | 0 |
| $Ni_3S_2$ | 0 | 0 | 0 |
| $NiMo_3S_4$ | 0.050 | 0.097 | 0.117 |

| Dopant Site | Supercell Size | LDA | PBE | PBE + GD2 |
|---|---|---|---|---|
| Mo subs. | $1 \times 1$ | 0.149 | 0.136 | 0.173 |
| | $2 \times 2$ | 0.107 | 0.102 | 0.107 |
| | $3 \times 3$ | 0.054 | 0.049 | 0.052 |
| | $4 \times 4$ | 0.031 | 0.281 | 0.030 |
| S subs. | $1 \times 1$ | 0.173 | 0.221 | 0.200 |
| | $2 \times 2$ | 0.090 | 0.084 | 0.086 |
| | $3 \times 3$ | 0.039 | 0.036 | 0.037 |
| | $4 \times 4$ | 0.022 | 0.021 | 0.021 |
| t-intercal. | $1 \times 1$ | 0.025 | 0.089 | 0.049 |
| | $2 \times 2$ | 0.002 | 0.024 | 0.015 |
| | $3 \times 3$ | 0.001 | 0.012 | 0.007 |
| | $4 \times 4$ | 0.001 | 0.007 | 0.004 |
| o-intercal. | $1 \times 1$ | 0.116 | 0.219 | 0.167 |
| | $2 \times 2$ | 0.044 | 0.062 | 0.049 |
| | $3 \times 3$ | 0.021 | 0.012 | 0.023 |
| | $4 \times 4$ | 0.012 | 0.018 | 0.013 |

**Table S4: Formation energies (eV/atom) w.r.t. bulk elemental phases for $\Delta\mu_{\mathrm{S}} = 0$, $\Delta\mu_{\mathrm{Mo}} = 0$, $\Delta\mu_{\mathrm{Ni}} = 0$**

| Formula | LDA | PBE | PBE + GD2 |
|---|---|---|---|
| Mo | 0 | 0 | 0 |
| Ni | 0 | 0 | 0 |
| S | 0 | 0 | 0 |
| $MoS_2$ | -1.023 | -0.890 | -0.872 |
| $Mo_3S_4$ | -0.812 | -0.689 | -0.623 |
| $Ni_2Mo$ | -0.203 | -0.112 | -0.109 |
| $Ni_3Mo$ | -0.160 | -0.078 | -0.079 |
| $Ni_4Mo$ | -0.174 | -0.082 | -0.082 |
| $NiS_2$ | -0.461 | -0.249 | -0.292 |
| $Ni_3S_4$ | -0.549 | -0.347 | -0.367 |
| NiS | -0.538 | -0.342 | -0.360 |
| $Ni_9S_8$ | -0.559 | -0.370 | -0.376 |
| $Ni_3S_2$ | -0.520 | -0.332 | -0.335 |
| $NiMo_3S_4$ | -0.755 | -0.591 | -0.557 |

| Dopant Site | Supercell Size | LDA | PBE | PBE + GD2 |
|---|---|---|---|---|
| Mo subs. | $1 \times 1$ | -0.593 | -0.444 | -0.409 |
| | $2 \times 2$ | -0.846 | -0.710 | -0.693 |
| | $3 \times 3$ | -0.938 | -0.807 | -0.788 |
| | $4 \times 4$ | -0.975 | -0.843 | -0.824 |
| S subs. | $1 \times 1$ | -0.645 | -0.475 | -0.481 |
| | $2 \times 2$ | -0.883 | -0.757 | -0.738 |
| | $3 \times 3$ | -0.962 | -0.832 | -0.814 |
| | $4 \times 4$ | -0.989 | -0.858 | -0.839 |
| t-intercal. | $1 \times 1$ | -0.861 | -0.677 | -0.694 |
| | $2 \times 2$ | -0.982 | -0.831 | -0.820 |
| | $3 \times 3$ | -1.005 | -0.862 | -0.849 |
| | $4 \times 4$ | -1.013 | -0.874 | -0.859 |
| o-intercal. | $1 \times 1$ | -0.769 | -0.547 | -0.575 |
| | $2 \times 2$ | -0.940 | -0.793 | -0.787 |
| | $3 \times 3$ | -0.985 | -0.862 | -0.832 |
| | $4 \times 4$ | -1.002 | -0.864 | -0.849 |

**Table S5: Formation energies (eV/atom) w.r.t. bulk elemental phases for $\Delta\mu_{\mathrm{Ni}} = 0$ and S-rich (Mo-rich) conditions**

| Formula | LDA | PBE | PBE + GD2 |
|---|---|---|---|
| Mo | 3.070 (0) | 2.670 (0) | 2.615 (0) |
| Ni | 0 (0) | 0 (0) | 0 (0) |
| S | 0 (1.535) | 0 (1.335) | 0 (1.308) |
| $MoS_2$ | 0 (0) | 0 (0) | 0 (0) |
| $Mo_3S_4$ | 0.504 (0.065) | 0.455 (0.074) | 0.498 (0.124) |
| $Ni_2Mo$ | 0.821 (-0.203) | 0.778 (-0.112) | 0.762 (-0.109) |
| $Ni_3Mo$ | 0.607 (-0.160) | 0.590 (-0.078) | 0.575 (-0.079) |
| $Ni_4Mo$ | 0.440 (-0.174) | 0.452 (-0.082) | 0.441 (-0.082) |
| $NiS_2$ | -0.461 (0.563) | -0.249 (0.641) | -0.292 (0.580) |
| $Ni_3S_4$ | -0.549 (0.329) | -0.347 (0.416) | -0.367 (0.380) |
| NiS | -0.538 (0.229) | -0.342 (0.326) | -0.360 (0.294) |
| $Ni_9S_8$ | -0.559 (0.163) | -0.370 (0.258) | -0.376 (0.239) |
| $Ni_3S_2$ | -0.520 (0.094) | -0.332 (0.202) | -0.335 (0.188) |
| $NiMo_3S_4$ | 0.396 (0.012) | -0.410 (0.076) | 0.423 (0.096) |

| Dopant Site | Supercell Size | LDA | PBE | PBE + GD2 |
|---|---|---|---|---|
| Mo subs. | 1 × 1 | -0.081 (0.430) | 0.001 (0.446) | 0.027 (0.463) |
| | 2 × 2 | 0.050 (0.178) | 0.068 (0.180) | 0.070 (0.179) |
| | 3 × 3 | 0.028 (0.085) | 0.034 (0.083) | 0.035 (0.084) |
| | 4 × 4 | 0.017 (0.049) | 0.020 (0.048) | 0.021 (0.048) |
| S subs. | 1 × 1 | 0.378 (0.122) | 0.416 (0.193) | 0.391 (0.173) |
| | 2 × 2 | 0.141 (0.077) | 0.133 (0.077) | 0.133 (0.079) |
| | 3 × 3 | 0.061 (0.033) | 0.058 (0.033) | 0.058 (0.034) |
| | 4 × 4 | 0.035 (0.019) | 0.033 (0.019) | 0.032 (0.019) |
| t-intercal. | 1 × 1 | 0.017 (0.017) | 0.086 (0.086) | 0.053 (0.053) |
| | 2 × 2 | 0.0001 (0.0001) | 0.024 (0.024) | 0.016 (0.016) |
| | 3 × 3 | 0.0001 (0.0001) | 0.012 (0.012) | 0.007 (0.007) |
| | 4 × 4 | 0.0002 (0.0002) | 0.007 (0.007) | 0.004 (0.004) |
| o-intercal. | 1 × 1 | 0.108 (0.108) | 0.216 (0.216) | 0.172 (0.172) |
| | 2 × 2 | 0.042 (0.042) | 0.062 (0.062) | 0.050 (0.050) |
| | 3 × 3 | 0.020 (0.020) | 0.012 (0.012) | 0.024 (0.024) |
| | 4 × 4 | 0.011 (0.011) | 0.017 (0.017) | 0.014 (0.014) |

**Table S6: Formation Energies with Vacancy Structures as References**

| eV | Mo subst. | S subst. |
|---|---|---|
| 2×2 | -2.544 | 0.092 |
| 3×3 | -2.609 | 0.159 |
| 4×4 | -2.584 | 0.162 |

Formation energies calculated for substitutional doping by filling a vacancy. Energies were calculated using: $E_{\text{form}} = E_{\text{doped}} - E_{\text{vacancy}} - E_{\text{Ni}}$. Mo substituted structures are calculated from Mo vacancies that are filled with a Ni atom. S vacancies are calculated from S vacancies filled with Ni.

**Table S7: Newly Active Modes in Raman/IR Spectra for 3×3 Mo Substitution**

| Classif. | Freq. ($cm^{-1}$) | Activity | Description |
|---|---|---|---|
| New peak | 60.92 | R/I | In doped layer: in-plane, Mo, S, and Ni; S in-phase |
| | 131.46 | R/I | In doped layer: in-plane Mo, S, Ni |
| | 132.40 | R/I | S out-of-phase some $z$-direction and some in-plane |
| | 161.97 | R/I | Around dopant: Ni-Mo in-plane and S $z$-direction |
| | 266.09 | R | Around dopant: Ni in-plane and Ni-S symmetric stretching |
| | 301.00 | R/I | In doped layer: S out-of-phase |
| | 345.17 | I | In doped layer: S out-of-phase, in-plane |
| | 356.06 | I | S out-of-phase, in-plane |
| | 363.88 | R | In doped layer: in-plane 1st and 2nd S and Mo neighbors of Ni |
| | 370.37 | I | In doped layer: S in-phase, in-plane |
| Activation | 208.86 | R/I | In doped layer: Mixed $E_{1u}$, $A_{1g}$, $B_{1u}$, and $E^1_{2g}$ |
| | 223.87 | I | In doped layer: Mixed $E_{1u}$ and $E^1_{2g}$ |
| | 387.74 | I | In undoped layer: Mixed $E^1_{2g}$ and $E_{1u}$ ($x$) |
| | 389.33 | I | In undoped layer: Mixed $E^1_{2g}$ and $E_{1u}$ ($y$) |
| | 456.80 | R | In doped layer: Mixed $A_{2u}$ and $B^1_{2g}$-like mode |
| | 470.18 | I | In doped layer: Mixed $A_{2u}$ and $B^1_{2g}$-like mode |

"In-" and "out-of-phase" refer to two S planes within a layer.

**Table S8: Newly Active Modes in Raman/IR Spectra for 3×3 S Substitution**

| Classif. | Freq. ($cm^{-1}$) | Activity | Description |
|---|---|---|---|
| New peak | 327.17 | R | S out-of-phase between adjacent S planes, in- and out-of-plane, in-phase between layers |
| | 333.45 | R | In doped layer: S in-plane on doped S plane, out-of-plane in adjacent S plane |
| | 336.69 | R | In undoped layer: S in-phase between planes |
| Activation | 473.49 | R/I | $B_{2g}^1$-like only on undoped layer |

**Table S9: Newly Active Modes in Raman/IR Spectra for 3×3 T-Intercalation**

| Classif. | Freq. ($cm^{-1}$) | Activity | Description |
|---|---|---|---|
| New peak | 261.85 | I | S in-plane breathing mode near Ni |
| | 366.42 | R | In 1-bond layer: in-plane breathing mode around Ni |
| | 372.07 | R | In 3-bond layer: in-plane breathing mode S near Ni |
| | 434.90 | R/I | In 3-bond layer: Ni-S asymmetric stretching |
| | 452.44 | R | In 3-bond layer: Ni-S symmetric stretching and S out-of-plane |
| | 503.26 | R/I | In 1-bond layer: Ni-S bond stretching |
| Activation | 335.80 | R | In 1-bond layer: $E_{1g}$-like out-of-phase in $x/y$ |
| | 465.14 | R/I | In 1-bond layer: Mixed $A_{2u}$ and $B_{2g}^1$-like + Ni-S stretch in 3-bond layer |
| | 468.12 | R/I | In 3-bond layer: Mixed $A_{2u}$ and $B_{2g}^1$-like + Ni-S stretch in both layers |

**Table S10: Newly Active Modes in Raman/IR Spectra for 3×3 O-Intercalation**

| Classif. | Freq. ($cm^{-1}$) | Activity | Description |
|---|---|---|---|
| New peak | 212.48 | R | Mostly in far layer: breathing mode around Ni, Mo and S in-phase, in-plane and S mostly out-of-plane (away from Mo plane) |
| | 235.11 | R | In far layer: in-plane breathing mode, Mo and S out-of-phase |
| | 329.64 | R/I | Mostly out-of-plane breathing by S around Ni |
| | 360.58 | R | In close layer: in-plane breathing by S atoms in one layer |
| | 426.60 | R | Symmetric Ni-S stretch |
| Activation | 53.91 | I | In close layer: $E^2_{2g}$-like shearing mode and Ni plane-direction vibration ($x$) |
| | 59.14 | I | In close layer: $E^2_{2g}$-like shearing mode and Ni plane-direction vibration ($y$) |
| | 66.75 | R | $B^2_{2g}$-like layer breathing mode |
| | 134.82 | R | Mixed $B^2_{2g}$ near Ni and Ni $z$-direction |
| | 281.80 | I | $E_{2u}$-like mode ($x$) |
| | 281.83 | I | $E_{2u}$-like mode ($y$) |
| | 286.80 | R | $E_{1g}$-like mode ($x$) |
| | 286.83 | R | $E_{1g}$-like mode ($x$) |
| | 469.73 | R | $B^1_{2g}$-like mode |

"Close" and "far" layer refers to proximity to the Ni atom, which is 0.3 Å closer to one layer than the other.

# References


(S1) Wolfram Research Inc., Mathematica 12.1. 2020.

(S2) Jain, A.; Ong, S. P.; Hautier, G.; Chen, W.; Richards, W. D.; Dacek, S.; Cholia, S.; Gunter, D.; Skinner, D.; Ceder, G.; Persson, K. A. Commentary: The Materials Project: A materials genome approach to accelerating materials innovation. *APL Materials* **2013**, *1*, 011002.

(S3) Kutana, A.; Penev, E. S.; Yakobson, B. I. Engineering electronic properties of layered transition-metal dichalcogenide compounds through alloying. *Nanoscale* **2014**, *6*, 5820.
